# Supplementary material for: CodeNeRF: Disentangled Neural Radiance Fields for Object Categories
Source: arXiv:2109.01750 source file (2021-09-03)
Supplement: Supplementary file 1 [file 9supp.tex]

\section{Supplementary: Estimating the camera extrinsic}

\subsection{Look-at function}

Given the camera position $\bf{o}$ and the target position $\bf{t}$, we can discover the camera to world matrix($c2w$) as below. Also, for SRN data set, the world-up vector($\bf{w}$) is defined as (0, 0, 1). 

\begin{equation}
    \begin{split}
        \bf{b} &= \bf{o} - \bf{tar} \\
        \bf{b} &= \frac{\bf{b}}{||\bf{b}||} \\ 
        \bf{w} &= (0, 0, 1) \\
        \bf{r} &= \bf{w} \times \bf{b} \\
        \bf{r} &= \frac{\bf{r}}{||\bf{r}||} \\
        \bf{u} &= \bf{b} \times \bf{r} \\
        c2w &= [\bf{r}|\bf{u}|\bf{b}|\bf{o}]
    \end{split}
\end{equation}

Here, we assume that the camera is initially placed at $(0, 0, r)$ where $r$ is the radius(the norm of the translation). 

Then, the given the camera position $bf(o)$ (and implicitly assume that $bf(t)= (0,0,0)$), we first discover $R(3,1), R(3,2), R(3,3)$ of rotation matrix through $\bf{o}=-R^T \bf{tar}$. 

Here, we assume that the world-up vector is $(0,0,1)$, which means the the $(1,0,0)$ of the  camera coordinate is always on $z=0$, so $R(1,3) = 0$ and we find $R(1,1), R(1,2)$ from the cross product and normalization, then we can discover $R(2,1), R(2,2), R(2,3)$ by the cross product as in the above equation.

\subsection{Axis-Angle Representation and Translation}

Given $k=(k_x,k_y,k_z) \in R^3$, which is unit vector, we can make the skew-symmetric matrix $K$. According to Rodriguez' rotation formula, we get $R =I+\sin(\theta)K + (1-\cos(\theta)K^2$. We have two degree of freedom at $k$, and one degree of freedom of $\theta$, and the 3 degree of freedom from the translation $\bf{t}$. $T_{wc} = [R|t]$. Here, we need $T_{cw} = [R^T|-R^T t]$. 

\paragraph{Explaining Look-at in this frame} We first assume that the translation vector is always on z-axis $\bf{t} = (0,0,r)$. Then, from the position of the camera $o$, we can find the $R[3,1], R[3,2], R[3,3]$, along with where the $z$-axis heads in the camera coordinate. Similarly, as in the above case, we assume that the $(1,0,0)$ of the camera coordinate is on the $z$-axis of the world coordinate. This could be achieved by below condition.

\begin{equation}
    \cos(\theta) = \frac{k_x^2 k_z^2 - k_y^2}{k_x^2 k_z^2 + k_y^2}
\end{equation}

What I have implemented so far is that we assume $\theta$ has certain value under the Rodriguez representation, along with the camera initially positioned at $(0, 0, r)$ then moved by the rotation matrix and the translation matrix.
